# Supplementary material for: Latent Representation and Simulation of Markov Processes via Time-Lagged Information Bottleneck
Source: arXiv:2309.07200 source file (2024-01-26)
Supplement: Supplementary file 1 [file data.tex]

\section{Data Details}

% We analyze trajectories obtained by simulating a molecule of \textit{Alanine Dipeptide} and two fast-folding mini-proteins, namely \textit{Chignolin} and \textit{Villin} \citep{Lindorff11}. For each molecule, we define disjoint \textit{train}, \textit{validation} and \textit{test} splits. The Alanine Dipeptide splits correspond to separate simulations of 250K/100K/100K frames, while Chignolin and Villin simulations involve splitting a single trajectory into three temporally disjoint parts: 334.743/100K/100K frames for Chignolin and 427.907/100K/100K frames for Villin. Each observation $\rvx_t$ consists of the set of the Euclidean coordinates of all the atoms and a one-hot encoding corresponding to the atomic number for the Alanine Dipeptide trajectories. The mini-proteins, on the other hand, are characterized by a coarse-grained representation representing the location of amino acids in the protein chain (10 for Chignolin and 35 for Villin), along with a one-hot encoding for the amino acid type. The temporal gap between consecutive frames is $1 ps$ for Alanine Dipeptide simulations and $200 ps$ for the mini-proteins. We generate targets $\rvy_t$ by clustering the TICA representation using KMeans as depicted in Figure~\ref{fig:representations}. Additional results for labels generated by discretizing different features are reported in the supplementary material. We choose a training lagtime $\tau$ for each molecule that is long enough to capture metastable state transitions, as shown in Figure~\ref{fig:autoinfo}
